# Supplementary material for: Strong spin-phonon coupling unveiled by coherent phonon oscillations in Ca2RuO4
Source: arXiv:1712.03028 source file (2018-06-25)
Supplement: Supplementary file 1 [file supplementary_material.pdf]

*Supplemental material* for

# Strong Spin-Phonon Coupling Unveiled by Coherent Phonon Oscillations of $Ca_2RuO_4$

Min-Cheol Lee[1, 2], Choong H. Kim[1, 2], Inho Kwak[1, 2], C. W. Seo[1, 3], Changhee Sohn[1, 2], F. Nakamura[4], C. Sow[5], Y. Maeno[5], E.-A. Kim[6], T. W. Noh[1, 2*] & K. W. Kim[3†]

[1]*Center for Correlated Electron Systems, Institute for Basic Science (IBS), Seoul 08826, Republic of Korea*

[2]*Department of Physics and Astronomy, Seoul National University, Seoul 08826, Republic of Korea*

[3]*Department of Physics, Chungbuk National University, Cheongju, Chungbuk 28644, Republic of Korea*

[4]*Department of Education and Creation Engineering, Kurume Institute of Technology, Fukuoka 830-0052, Japan*

[5]*Department of Physics, Graduate School of Science, Kyoto University, Kyoto 606-8502, Japan*

[6]*Department of Physics, Cornell University, Ithaca, New York 14853, USA*

Corresponding authors:

[*]twnoh@snu.ac.kr, [†]kyungwan.kim@gmail.com

# 1. Methods

## Experimental methods

We perform photoinduced reflectivity measurements on single crystals of $Ca_2RuO_4$ that are synthesized using the floating zone method [1]. We cleave the crystals immediately prior to the optical experiments. We use a commercial Ti:sapphire amplifier at a 250 kHz repetition rate. The center wavelength is 800 nm, and the pulse width is 30 fs. Although the pump fluence dependent measurements show a linear response of the coherent phonon oscillations over a wide fluence range beyond 1 mJ/cm$^2$, we present data measured at the laser fluences to 140 μm/cm$^2$ and 80 μm/cm$^2$. The spot sizes for the pump and probe pulses are 80 μm and 40 μm (FWHM), respectively. The pump and probe pulses are linearly polarized and perpendicular to each other and the sample does not exhibit anisotropy depending on both pump and probe polarizations.

## Density Functional Theory (DFT) calculations

Our first-principles calculations are performed based on DFT using the Perdew-Burke-Ernzerhof (PBE) form of the exchange correlation functional, as implemented in the Vienna Ab Initio Simulation Package [2,3]. We use an 8x8x4 k-point mesh and a kinetic energy cut-off value of 500 eV. We adopt $U_{\mathrm{eff}}$ (= $U - J$) = 2.5 eV to consider the local Hubbard interaction in Ru. For the structural relaxation, the Hellman–Feynman forces are converged to 0.5 meV/Å. To calculate the zone-center phonon mode, we use the frozen phonon method. To calculate the octahedral deformation depicted in Fig. 4, we have fully optimized internal coordinates including position of oxygen atom for antiferromagnetic (AFM) and ferromagnetic (FM) configurations with fixed the lattice constant data measured at finite temperatures (11 K) [4].

## 2. Fluence dependence of the coherent phonon oscillations

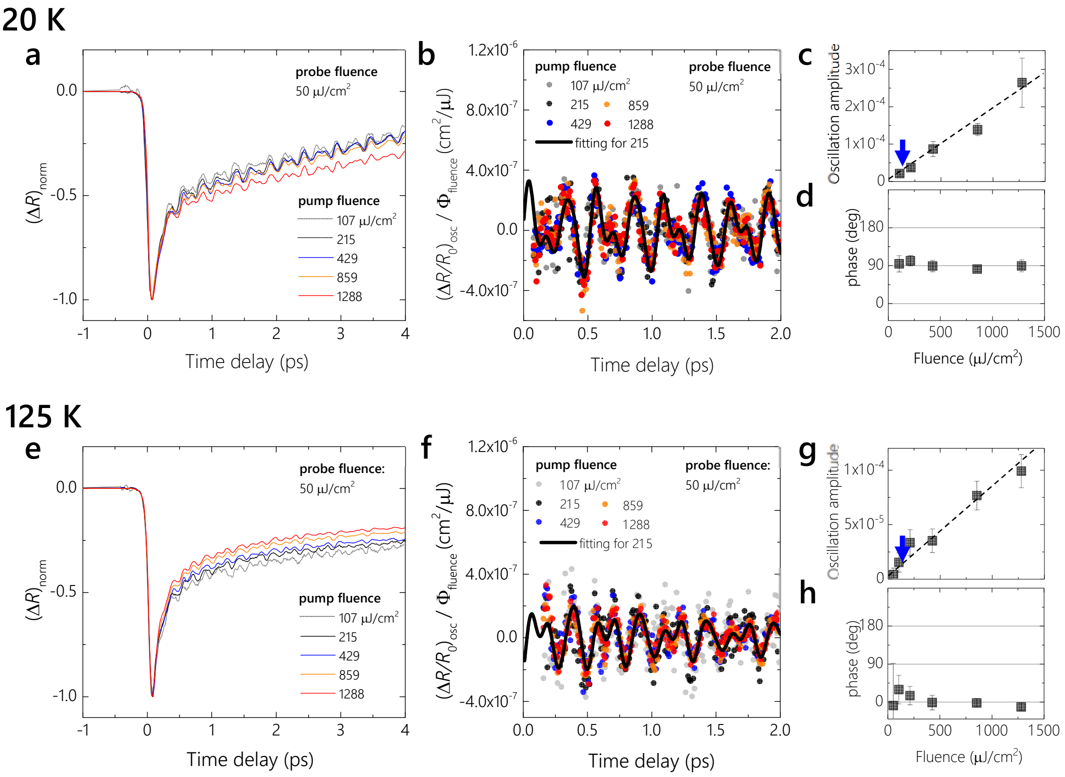


**Figure S1**. Fluence dependent reflectivity changes and coherent oscillations at 20 K (< $T_N$ = 113 K) and 125 K (> $T_N$). **(a), (e)** Photo-reflectivity normalized by the maximum value under pump fluence up to ~ 1 mJ/cm$^2$. **(b), (f)** Extracted oscillation components and a fitting curve composed of four $A_g$ modes. **(c), (g)** Amplitude and **(d), (h)** *phase* values of the lowest $A_g$ phonon oscillations under various pump fluence. It clearly shows a linear response at least up to ~ 1 mJ/cm$^2$. The blue arrow in (c) indicates the pump fluence that was used for measurements in the manuscript.

The oscillation-*phase* of the lowest $A_g$ phonon mode does not depend on light fluence. Fig. S1 shows the fluence dependent data of the coherent phonon oscillations at different temperatures of 20 K (< $T_N$) and 125 K (> $T_N$) with various pumping fluences. In particular, oscillation-*amplitude* of the lowest $A_g$ mode clearly show a linear response, and the oscillation-*phase* stays at the same value even at pumping fluence up to ~ 1 mJ/cm$^2$. Despite the linear response of the coherent phonon oscillations, we present data measured at pump and probe fluences of 140 μJ/cm$^2$ and 80 μJ/cm$^2$, respectively, to minimize heating effect and to stay close to a linear response region of the electronic response.

## 3. Fits to relaxation dynamics

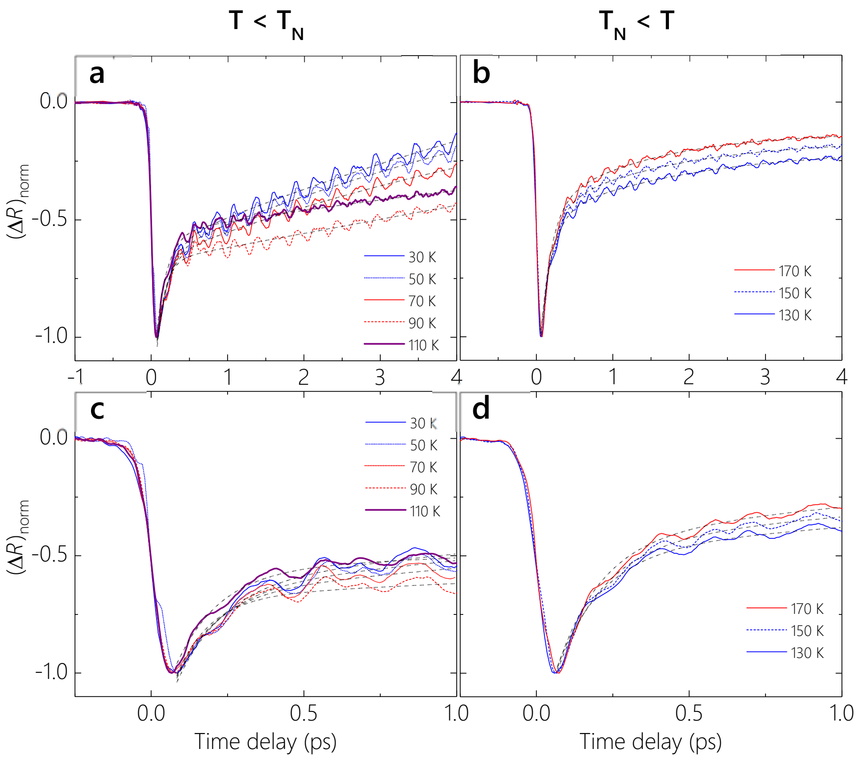


**Figure S2**. Relaxation fits (black dotted lines) of two-exponential decay model for temperature dependent reflectivity changes (colored lines)

We analyze the oscillatory components due to coherent phonons after subtracting double exponential decay function fits to the electronic response. Fig. S2 shows reflectivity change within few picoseconds and relaxation fits at various temperatures. Although there is gradual temperature-dependent evolution, the overall electronic response does not show an abrupt change across phase transitions that might influence the coherent oscillations under discussion.

## 4. Fits to coherent phonon oscillations

We fit the $A_g$ coherent phonon oscillations with a damped harmonic oscillating model given as:

$$R_{CP}(t) = -\Sigma_i A_i \cos(2\pi f_i + \phi_i) \exp(-t/\tau_i),$$

where $A_i$, $f_i$, $\phi_i$, and $\tau_i$ are the amplitude, frequency, initial *phase*, and damping time of the $A_g$ symmetric modes. We mainly consider four oscillators corresponding to the equilibrium $A_g$ Raman modes [5,6]. Fourier transform spectra in Fig. 3(b) barely reveal that there are two $A_g$ modes around 5.8 ~ 6 THz but we confirm by DFT calculations that these two modes are distinct with similar resonant energy. Therefore, we consider four modes including both modes around 6 THz in our model. The anomalies in *phase* and amplitude are first obtained by fitting all parameters of the four modes. Figure S3(a) and (b) show the fitting results. The oscillatory components of 3.8 THz mode in figure S3(a) are obtained by subtracting the fitting functions of other three modes from the raw data. Figure S4 shows the oscillation-*phases* of all four modes in the case of fitting without fixed *phase*s for all the $A_g$ modes. We find that not only the lowest frequency mode but also other modes show some variations. However, the fitting error bars are very large for parameters of other modes (Please note that the error bars here do not include the errors in the measurements). We also notice that the oscillation amplitudes of other modes are relatively small and their temperature dependences are not systematic. Therefore, we cannot trust the outcome as they are. With these results, one may suspect that such non-systematic fitting parameters could produce a systematic artifact in the other fitting parameter, that is, in the oscillation-phase of the 3.8 THz mode.

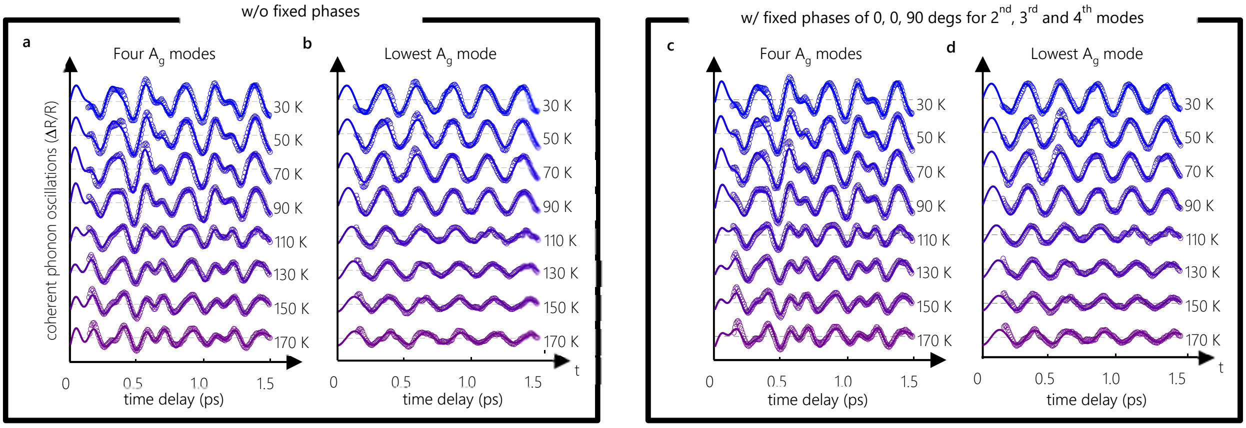


**Figure S3**. Fits for the lowest and other higher frequency $A_g$ coherent phonon modes (a, b) without and (c, d) with fixing the oscillation-*phase*s of higher frequency modes. (a) and (c) show the all oscillating components, and (b) and (d) show the lowest frequency component and fit functions after subtracting the fit functions of the other higher modes.

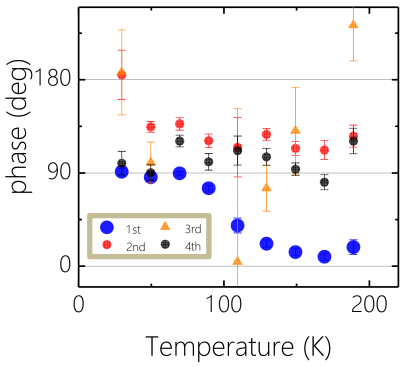


**Figure S4.** Oscillation-*phases* from the fits to the oscillatory signal.

Because the oscillation-*phase* is usually considered as a robust quantity of either 0 or 90 degrees depending on the generation mechanism, we repeat fitting with all the oscillation-phases fixed except the 3.8 THz mode. We have tried with the oscillation-*phases* of (0, 0, 0) degrees, (90, 90, 90) degrees, and (0, 0, 90) degrees for (5.8, 6.2, 7.5) THz modes, respectively. Among them, we find the condition of (0, 0, 90) degrees for (5.8, 6.2, 7.5) THz modes gives the best fitting quality, of which results are shown in figure S4(c), (d). We note that these phase angles are the values at the lowest temperature in Fig. S4 where the damping of all modes and the fitting error bars are smallest. We find that the overall fitting qualities with or without fixing the oscillation-*phases* are comparable.

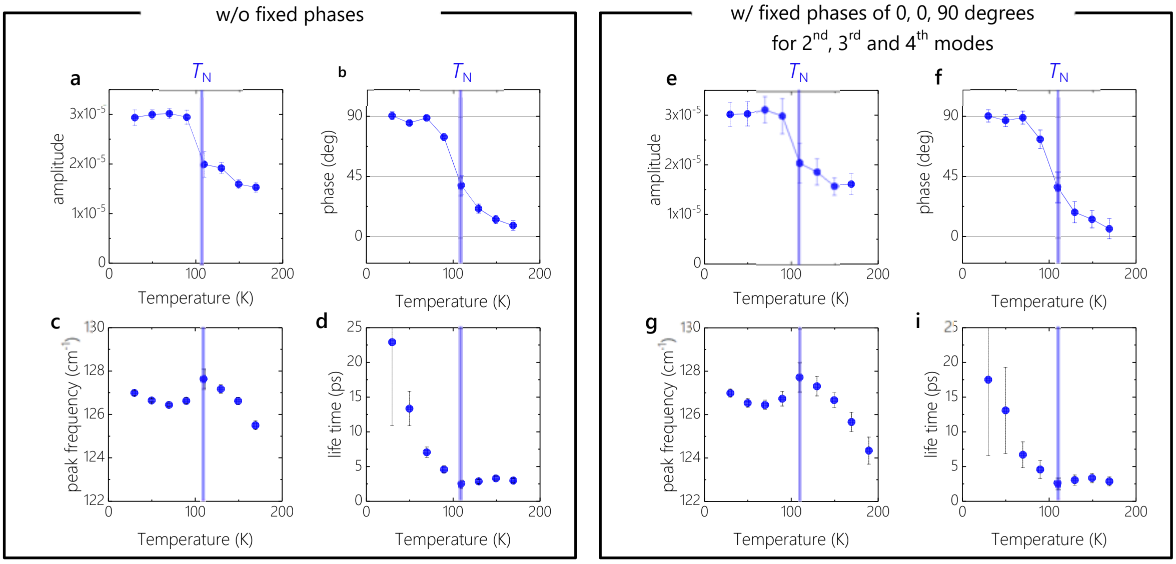


**Figure S5**. Fitting parameters of amplitude, *phase*, peak frequency and life time of the lowest frequency $A_g$ mode extracted by the damped harmonic oscillator models (a-d) without and (e-h) with fixing oscillation-*phase*s of higher frequency modes. It is clear that the *phase* values of the other modes do not influence the temperature dependent anomalies of the 3.8 THz $A_g$ mode.

Figure S5 shows the detailed parameters of the 3.8 THz mode from the two fitting results. It becomes clear that the anomalies in the 3.8 THz phonon modes do not depend on the fitting parameters of the other modes. Because it does not make a sense to allow the phases of all modes change randomly, we use the fitting result with fixing the oscillation-*phases* of other modes for the further discussions in the manuscript.

## 5. Theoretical models for coherent phonon oscillations

Here we introduce a microscopic model which has successfully explained the generation of coherent oscillations with random oscillation-*phases* [7–9]. The model assumed that the dielectric function $\tilde{\varepsilon} = \varepsilon_1 + i\varepsilon_2$ varies slowly within the bandwidth of the pump pulse. In addition, two-band approximation of the Raman susceptibility tensor was used. This results in the driving force of the oscillations as following:

$$F(t) \approx M\left[\frac{d\varepsilon_1}{d\omega}|E(t)|^2 + 2\varepsilon_2\int_{-\infty}^{t} e^{-\Gamma(t-t')}|E(t')|^2 dt'\right]. \quad (2)$$

where *M* is the matrix element of the electron-phonon coupling including a constant coefficient, *E*(*t*) is the electric field of the pump pulse, and Γ is the decay rate of the driving force. When the pulse duration is much shorter than the phonon oscillation period, the first term makes a total impulse $M\frac{d\varepsilon_1}{d\omega}\int_{-\infty}^{\infty}|E(t')|^2 dt'$ responsible for the impulsive oscillations, while the second term produces a displacive force after pumping. The cosine type oscillations in opaque materials can be explained by the second term with $\Gamma \ll \Omega$, which produces a constant force $2M\varepsilon_2\int_{-\infty}^{\infty}|E(t')|^2 dt'$ resulting in a displacive motion [7–9]. In general, both displacive and impulsive contributions can coexist, resulting in a random oscillation-*phase* such that $\Delta Q(t) = A\sin(\Omega t) + B\cos(\Omega t) = \sqrt{A^2+B^2}\cos(\Omega t + \phi)$. The relative ratio of the oscillation amplitudes *A*/*B* $= \frac{\Omega d\varepsilon_1/d\omega}{2\epsilon_2}$ determines the oscillation-*phase* of $|\phi| = arctan(|A/B|) = arctan\left(\left|\frac{\Omega d\varepsilon_1/d\omega}{2\epsilon_2}\right|\right)$ [7–9]. Therefore, the coherent oscillations with strong light absorption are dominantly by displacive contributions. From ellipsometry measurements on $Ca_2RuO_4$, we find that $\frac{d\varepsilon_1}{d\omega} \lesssim 2\ \mathrm{eV}^{-1}$ and $\frac{2\varepsilon_2}{\Omega} \sim 500\ \mathrm{eV}^{-1}$, as shown in Fig. S6. That is, the oscillations in $Ca_2RuO_4$ at all measured temperatures across the magnetic phase transition should be displacive cosine-type. We note that a fast decay of the displacive force with finite Γ, can result in a non-zero oscillation-*phase* of $|\phi| = arctan\left(\left|\frac{\Omega^2\frac{d\varepsilon_1}{d\omega}+2\Gamma\varepsilon_2}{\Omega\left(2\varepsilon_2-\Gamma\frac{d\varepsilon_1}{d\omega}\right)}\right|\right)$ [8].

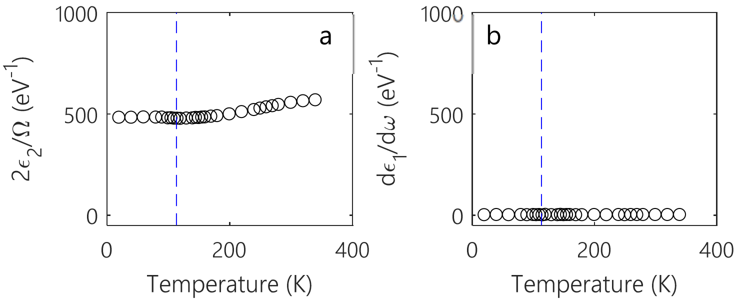


**Figure S6**. (a) $\frac{d\varepsilon_1}{d\omega}$ and (b) $\frac{2\varepsilon_2}{\Omega}$ at various temperatures in $Ca_2RuO_4$. The blue dotted lines indicate the spin ordering temperature of $T_N$ = 113 K. To obtain the dielectric constants, we measure the *ab*-plane reflectivity spectra from 20 K to 340 K using spectroscopic ellipsometry.

## 6. Determination of time zero delay

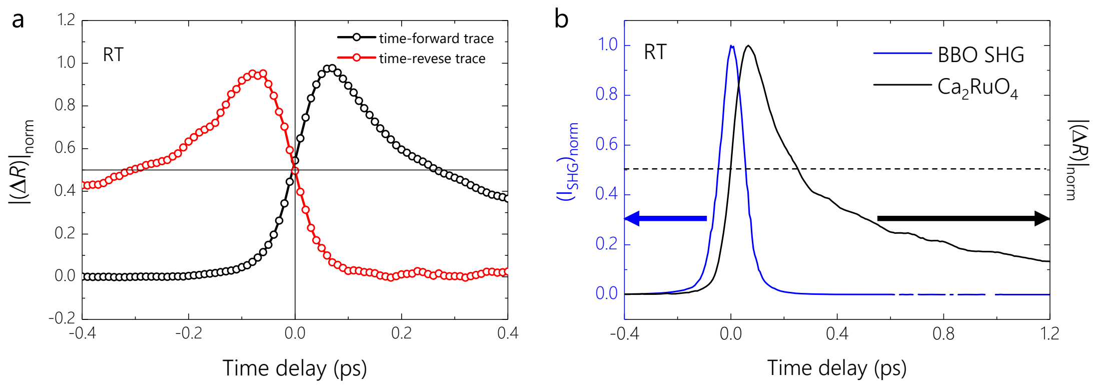


**Fig. S7**. (a) pump-probe data of $Ca_2RuO_4$ obtained by optical chopping the pump beam (black) and the probe beam (red). (b) second harmonic signal by pump and probe pulses from BBO (blue) crystal and the photo-reflectivity change of $Ca_2RuO_4$ (black). We measure all the data at room temperature, and display with the absolute values normalized by maximum changes for easy comparison.

The precise determination of the time zero is necessary to make a serious discussion on the oscillation-*phase*. We determine the time zero from (a) forward and backward traces of pump-probe signal, and (b) the cross correlation of pump and probe pulses as shown in figure S7. In the former case of (a), we chop the pump beam in the forward trace (black curve), and chop the probe beam in the backward trace (red curve) [10]. The latter case of (b) is obtained by the second harmonic signal of pump and probe pulses. Please note that although the time widths of both pump and probe pulses measured by a commercial autocorrelator (model: *PulseScout*, Newport Corporation) are 30 fs, the width of the cross correlation signal is a bit larger because we have used a thick (0.5 mm) beta barium borate (BBO) crystal for the second harmonic generation (SHG) measurement. The time error due to the specification of the delay stage is about 3 fs considering the reproducibility within 0.5 μm (model: M-IMS600LM, Newport Corporation). In practice, the maximum onset time variation among repeated measurements over 10 times was 10 fs, and this corresponds to 15-degrees-error in the oscillation-*phase* values.

## 7. Eigenmode of the lowest $A_g$ phonon oscillation

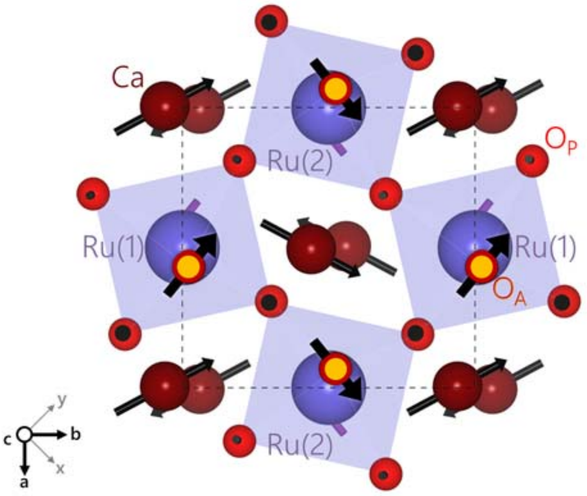


**Fig. S8.** Eigenmode of the lowest $A_g$ phonon mode obtained by DFT calculations. $O_P$, $O_A$, and Ru(1)/Ru(2) indicate the in-plane oxygen, apical oxygen and two sets of Ru ions.

We demonstrate the eigenmode of the lowest $A_g$ phonon mode by DFT calculation as shown in Figure S8. The mode is composed of ionic vibrations of $Ca^{2+}$ and $O^{2-}$ ions, while $Ru^{4+}$ ions have no displacement. Although the vibrational displacement of $Ca^{2+}$ is large, we mainly consider those of $O^{2-}$ in $RuO_6$ octahedral because it can directly couple to $Ru^{4+}$ orbital states and spin configuration. In the octahedral vibrations of $RuO_6$, the in-plane oxygen ($O_P$) show tilting distortions along *a*-axis, while the apical oxygen ($O_A$) show distortions along *y*/*x* directions in Ru(1)/Ru(2) ions.

## 8. Lattice deformation across the magnetic transition in $Ca_2RuO_4$

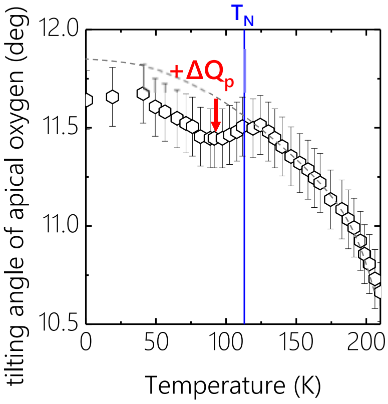


**Fig. S9** The tilting angle of apical oxygen at various temperatures extracted from previous neutron scattering results [4]. Grey dotted lines are guide for the thermal evolution. The red arrow indicates the decrease of tilting in the magnetic phase resulted from DFT calculations.

We also find an evidence of the structural distortion with the magnetic ordering from the previous neutron scattering data [4]. We extract the tilting angle of apical oxygen as a function of temperature as shown in Fig. S9. One can notice an anomaly across $T_N$, although it has not been pointed out before because the variation is comparable to the experimental error bars. In particular, the decrease of the tilting angle is in nice agreement with our DFT calculation results. Please note that the red arrow in Fig. S9 indicates the theoretically expected value of the angle change (0.15 degrees) from paramagnetic phase to antiferromagnetic phase.

## References


[1] S. Nakatsuji and Y. Maeno, J. Solid State Chem. **156**, 26 (2001).

[2] G. Kresse and J. Hafner, Phys. Rev. B **47**, 558 (1993).

[3] G. Kresse and D. Joubert, Phys. Rev. B **59**, 1758 (1999).

[4] M. Braden, G. André, S. Nakatsuji, and Y. Maeno, Phys. Rev. B **58**, 847 (1998).

[5] H. Rho, S. L. Cooper, S. Nakatsuji, H. Fukazawa, and Y. Maeno, Phys. Rev. B **71**, 245121 (2005).

[6] S.-M. Souliou, J. Chaloupka, G. Khaliullin, G. Ryu, A. Jain, B. J. Kim, M. Le Tacon, and B. Keimer, Phys. Rev. Lett. **119**, 067201 (2017).

[7] T. Stevens, J. Kuhl, and R. Merlin, Phys. Rev. B **65**, 144304 (2002).

[8] D. M. Riffe and A. J. Sabbah, Phys. Rev. B **76**, 085207 (2007).

[9] J. J. Li, J. Chen, D. A. Reis, S. Fahy, and R. Merlin, Phys. Rev. Lett. **110**, 047401 (2013).

[10] H. J. Zeiger, J. Vidal, T. K. Cheng, E. P. Ippen, G. Dresselhaus, and M. S. Dresselhaus, Phys. Rev. B **45**, 768 (1992).
